# Supplementary material for: Surface Defect Identification using Bayesian Filtering on a 3D Mesh
Source: arXiv:2501.18315 source file (2025-01-30)
Supplement: Supplementary file 1 [file appendix.tex]

\section{Appendix}
\subsection{Solution of the polygonal mesh problem} \label{sec:optsol}
The final goal of the algorithm is to estimate the \textit{dissimilarity} of the measured object w.r.t. the reference provided by the CAD model;
to this extend, we consider a state $\vec x \in \mathbb R^{n_v}$ representing deviation index of the object under inspection given the reference model.

In particular we assign to each vertex $\overline{\vec V}_i$ of the CAD a direction $\vec n_i \in \mathbb R^3$ with respect to which the error is projected; let $x_i$ be $i$-th component of $\vec x$, then the point subjected to such state moves to
\begin{equation} \label{eq:normalincrease}
    \vec V_i = \overline{\vec V}_i + x_i \vec n_i.
\end{equation}

In our case the choice of $\vec n_i$ is strongly related to the topology of the expected object shape. Considering that topological defects that can be observed in 3D are normal to the surface of the object, it is reasonable to chose $\vec n_i$ \textit{as normal as possible} to the polygonal shape. More formally, let $\mathcal N_i \subset \mathbb N$ the set of vertex indexes that have a connection with the $i$-th vertex, we chose
\begin{equation} \label{eq:normal_opt_problem}
\begin{aligned}
    \vec n_i = && \arg\min_{\vec n} \quad & c(\vec n) = \sum_{j \in \mathcal N_i} \left( \vec d_{ij}^\top  \vec n\right)^2\\
    && \textrm{subject to} \quad & \| \vec n\|^2 = 1
\end{aligned}
\end{equation}
where $\vec d_{ij} = \vec V_i - \vec V_j$; in Sec. \ref{sec:optsol} a solution of the problem is reported.
The solution of (\ref{eq:normal_opt_problem}) can be found using Lagrange multipliers for constrained optimisation problem. Let $\lambda \in \mathbb R$ the Lagrange multiplier of the constraint, then problem (\ref{eq:normal_opt_problem}) is equivalent to
\begin{equation}
    \arg\min_{\vec n, \lambda} \quad  c (\vec n, \lambda)= \sum_{j \in \mathcal N_i} \left( \vec d_{ij}^\top  \vec n\right)^2 + \lambda (\vec n^\top \vec n - 1).
\end{equation}
The first-order condition requires that the gradient of the cost function $c$ w.r.t. the decision variables $\vec y = (\vec n^\top, \lambda)^\top \in \mathbb R^4$ is zero:
\begin{equation} \label{eq:firstordcond}
    \vec f(\vec y) = \frac{\partial c}{\partial \vec y} = \begin{pmatrix}
        2 \left(\mat D +\lambda \mat I\right) \vec n \\
        \vec n^\top \vec n - 1
    \end{pmatrix} = 0 \in \mathbb R^4
\end{equation}
where
\[ \mat D = \sum_{j \in \mathcal N_i} \vec d_{ij} \vec d_{ij}^\top \in \mathbb R^{3\times 3}. \]
Since (\ref{eq:firstordcond}) is a non-linear set of equation, an approximate solution can be found with Newton's iterative method
\begin{equation}
    \vec y^{(k+1)} = \vec y^{(k)} - \mat J^{-1}\big( \vec y^{(k)}\big) \vec f \big( \vec y^{(k)} \big),
\end{equation}
with the Jacobian matrix $\mat J \in \mathbb R^{4\times4}$ being
\begin{equation}
    \mat J(\vec y) = \begin{bmatrix}
        2(\mat D + \lambda \mat I) & 2\vec n \\ 2\vec n^\top & 0
    \end{bmatrix}.
\end{equation}
At convergence of the algorithm it is also possible to check that indeed the point is a local minima (and not a maxima) by checking if $\mat J$, that's actually the hessian of the cost function $c$, is positive definite (or not).

\subsection{Extended information filter}
The extended information filter uses a transformation to move from the \textit{uncertainty domain} characterized by $\vec \mu, \mat \Sigma$ to an \textit{information domain} characterized by $\vec \xi, \mat \Omega$.  Given that transformations are
\begin{equation}
    \mat \Sigma = \mat \Omega^{-1} \qquad \vec \mu = \mat \Omega^{-1} \vec \xi,
\end{equation}
then each call on the WLS algorithm becomes
\begin{align}
    \mat \Omega_{k+1} & = \mat H_k^\top \mat R_k^{-1} \mat H_k + \mat \Omega_k \\
    \vec \xi_{k+1} & = \mat H_k^\top \mat R_k^{-1} \vec z_k + \vec \xi_k
\end{align}
This operations are numerically less expensive (product of sparse matrices).
The lonely issue is to return to $\vec \xi, \mat \Sigma$ since it requires the inversion of $\mat \Omega$ that in general is big.
Still this operation can be performed only few times.
